# Supplementary material for: Multiplayer Multi-armed Bandits for Optimal Assignment in Heterogeneous Networks
Source: arXiv:1901.03868 source file (2019-08-30)
Supplement: Supplementary file 1 [file Appendix.tex]

\section*{Proof of Lemma \ref{lma:secondAlloc}}
Let $\hat{M}(l)$ be the estimated matrix after learning and signalling in the $l^{th}$ epoch. Let $\hat{\pi}_1(l) \in A(\hat{M}(l))$ and $\hat{\pi}_2(l) \in \bar{A}(\hat{M}(l))$ be a best and a second-best allocations on $\hat{M}(l)$ respectively. Let $\pi_1$ and $\pi_2$ be similar quantities in case of the matrix $M$.
Also, we define $\hat{\Delta}_{min}(l) = f(\hat{M}(l),\hat{\pi}_1(l)) - f(\hat{M}(l),\hat{\pi}_2(l))$. Also, let $I$ be an all ones matrix.

\textit{Case 1}: If $\pi_1=\hat{\pi}_1$, $f(\hat{M},\hat{\pi}_2) \leq f(M+\epsilon I,\hat{\pi}_2) \leq f(M+\epsilon I,\pi_2)$
where the second inequality holds because $\pi_1=\hat{\pi}_1 \neq \hat{\pi}_2$ and thus $\hat{\pi}_2$ cannot give better reward on $M$ than $\pi_2$. 

\textit{Case 2}: If $\pi_1 \neq \hat{\pi}_1$,
$f(\hat{M},\hat{\pi}_2) \leq f(\hat{M},\hat{\pi}_1) \leq f(M+I\epsilon,\hat{\pi}_1) \leq f(M+I\epsilon,\pi_2)$ where the last inequality holds because $\pi_1 \neq \hat{\pi}_1$ and thus $\hat{\pi}_1$ cannot give better reward than $\pi_2$ on $M$. \\
$ \because f(M+\epsilon I,\pi_2) = f(M,\pi_2)+N\epsilon$, $f(\hat{M},\hat{\pi}_2) - f(M,\pi_2) \leq N\epsilon$.

A similar comparison of $\hat{M}$ with $M-\epsilon I$ instead of $M + \epsilon I$ proves that $f(M,\pi_2) - f(\hat{M},\hat{\pi}_2) \leq N\epsilon $. 

We thus obtain $-2N\epsilon \leq \Delta_{min} - \hat{\Delta}_{min} \leq 2N\epsilon$ from equation (\ref{eqn:perturb2}) and the above equation.  \hfill \IEEEQED

\section*{Proof of Theorem \ref{thm:mESER}}
 
We continue to prove the regret bound similar to the way it was done for Theorem 2 in \cite{TCNS2018_DecentralizedLearning_KalthilNayyarJain}. We provide bounds on the regret in the 3 phases of exploration ($R^{0}(T)$) , signalling($R^{S}(T)$) and exploitation($R^{E}(T)$). 

In the exploration phase, every epoch has $T_s(l) = 8N^2log^{(\beta)}(t_l)$ time slots till the $l_1^{th}$ epoch after which it is a constant equal to $T_0$, giving a total regret of 
\begin{equation*}
\begin{array}{lcl}
R^O(T) 
&\leq &\sum_{l=1}^{l=l_1} \Delta_{max} T_s(l)K + \sum_{l=l_1+1}^{l=l_0} \Delta_{max} T_s(l_1)K\\
& \leq & \Delta_{max}Klog(t_{l_1})T_s(l_1) +\Delta_{max} T_0Klog(T) \\
& \leq & \Delta_{max}KC_1 +\Delta_{max} T_0Klog(T) \\
\end{array}
\end{equation*}

Similarly for the signalling phase, we consider packetized transmission. If $T_b(l) = \lceil log_2(4N/(\epsilon(l)) \rceil$, we can see that $T_b(l) \leq log_{2}(4N) + log^{\beta/2}(t_l)$. Also, $\forall l > l_1$, $T_b(l) =T_1=\lceil log_2(4N/(\epsilon_0) \rceil$. Thus we have the regret in the communication phase as  
\begin{equation*}
\begin{array}{lcl}
R^{S}(T) 
& \leq &  \sum_{l=1}^{l=l_0}T_b(l) KN^2 =  N^2K \sum_{l=1}^{l=l_0}T_b(l) \\
& \leq & N^2K \sum_{l=1}^{l=l_1}T_b(l) + N^2K \sum_{l=l_1}^{l=l_0}T_b(l_1) \\
&  \leq & N^2K( log_2(4N)l_1 + log^{(1+\beta)}(t_{l_1})) + N^2KT_1log(T)  \\
&  = & N^2KC_2 + N^2KT_1log(T)  \\
\end{array}
\end{equation*}
We now look at the regret in the exploitation phase. Over the $l^{th}$ epoch, the expected regret would be $R^E(l) \leq 2^{l}(\epsilon(l)(1-\delta(l) + \Delta_{max}\delta(l))$. After $l_1$ epochs, we set $\epsilon(l) = \epsilon_0 < \Delta_{min}$. Thus the overall regret $R^{E}(T) = \sum^{l_0}_{l=1}R^E(l)$ would be:
\begin{equation*}
    \begin{array}{lcl}
    R^{E}(T) 
    & \leq & \sum^{l_1}_{l=1}2^{l}(\epsilon(l)+\delta(l)(\Delta_{max}-\epsilon(l)))\\
    &  & + \Delta_{max}\sum^{l_0}_{l=l_1+1}2^{l}\delta(l)= R^{E}_1(T) + R^{E}_2(T)\\
    R^{E}_1(T) 
    & = & \sum^{l_1}_{l=1}2^{l}(\epsilon(l)+\delta(l)(\Delta_{max}-\epsilon(l)))\\
    & \leq & 2^{l_1+1}(1+\Delta_{max}) = C_3\\
    R^E_2(T)
    &= & \Delta_{max}\sum^{l_0}_{l=l_1+1}2^lPr\{ |\hat{M}(l)>M|>\epsilon(l)/2N  \}\\
    & \leq & \Delta_{max}\sum^{l_0}_{l=l_1+1}2^{l}*3NKe^{-\epsilon(l)^2lT_s/8N^2}\\
    & \leq & 3NK\Delta_{max}\sum^{l_0}_{l=l_1+1}(2e^{-\epsilon_0^2T_s/8N^2})^{l}\\
    & \leq & 3NK\Delta_{max}\sum^{\infty}_{l=l_1+1}(2e^{-1})^{l} = C_4NK\Delta_{max}\\
\end{array}
\end{equation*}

where $C_4 = 3r^{l_1}/(1-r)$ and $r=2e^{-1}$. \hfill \IEEEQED

\section*{Proof of Lemma (\ref{lma:RHPhase})} 
Let $p_c$ denote the collision
probability of a player when all the players are randomly selecting an arm to play from $[K]$ in each round. Probability that each a player  will observe a collision-free play on an arm after  $T_{01}$ rounds is given by:
\[\sum_{t=1}^{T_{01}}p_c^{t-1}(1-p_c).\]
Setting this value to be at least larger than $1- \frac{\delta}{N}$ for each player we get
\begin{eqnarray}
	\lefteqn{\sum_{t=1}^{T_{01}} p_c^{t-1}(1-p_c) \geq 1- \frac{\delta}{3N}} \nonumber\\
	&\iff&1-{p_c}^{T_{01}} \geq 1- \frac{\delta}{3N} \nonumber \\
	&\iff& T_{01} \log{p_c} \leq \log\bigg({\frac{\delta}{3N}}\bigg) \nonumber \\
	&\iff& T_{01} \geq \frac{\log\big({\frac{\delta}{3N}}\big)}{\log{p_c}} \label{eqn:TRHBound}.
\end{eqnarray}
We next give an uniform upper bound on $p_c$. Note that in any round some players may be already locked (call locked players) while others still selecting uniformly at random (call them RH players). Fix a round $t$ and let $N_r \geq 1 $ denote the number of RH players. Let $p_{cr}$ denote the probability that collision is observed from a RH player. We have

\begin{eqnarray*}
	\lefteqn{1-p_c= \Pr\{\mbox{no colision from RH players}\}} \\
	&+& \Pr\{\mbox{no colision from locked players}\} \\
	&\geq & \sum_{j=1}^{N_r}(1-p_{cr})/K\geq (1-p_{cr})/K \\
	&=& (1-1/K)^{N_r-1}/K\\
	&\geq& (1-1/K)^{N-1}/K\geq 1/4K (\mbox{ for all } K>1).
\end{eqnarray*}  

Substituting the bound on $p_c$ in (\ref{eqn:TRHBound}) and using union bound we see that within
$ T_{r}$ rounds all the players will orthogonalize with probability at least $1-\delta/3$. \hfill\IEEEQED

\section*{Proof of Lemma (\ref{lma:SHPhase})}
The proof from a straightforward application of Hoeffding's inequlaity. Recall that in SH phase there will be no collision and players will observe a reward sample in each round. Fix a player $n \in [N]$. We have 

\begin{eqnarray*}
\lefteqn{\Pr\left \{\exists k \in [K] \mbox{ such that  } |\mu_{n,k}-\hat{\mu}_{n,k}|\geq \epsilon/4N\right \}} \\  &\leq\sum_{k \in [K]}\Pr\{ |\mu_{n,k}-\hat{\mu}_{n,k}|\geq \epsilon/4N\}\\
& \leq \sum_{k \in [K]} 2 \exp\left \{- 2T_s(\epsilon/4N)^2 \right \}\\
&= \sum_{k \in [K]} 2\exp\{-\log(6NK/\delta)\}= \delta/3N,
\end{eqnarray*}
where the first inequality follows the union bound, the second form Hoeffding's inequlaity, and the last from substituting value of $T_s$ given in (\ref{eqn:SHLen}). Applying union bound  over all the players we get
\[\Pr\left \{\forall \; n\in [N],  k\in [K], \;\;|\mu_{n,k}-\hat{\mu}_{n,k}\;\; |\leq  \epsilon/4N\right \}> 1- \delta/3\]
\hfill\IEEEQED

\section*{Proof of Lemma (\ref{lma:BSPhase})}
In the BS phase players $n \in [N]$ transmit with probability $\hat{\mu}_{n,j}$ for $T_b$ number of rounds for each $j \in [K]$ on an arm while all the other players listen on it. The probability that each entry in the $k$th column of $\hat{M}$ is not estimated within $\epsilon/(2N)$ accuracy is bounded as

\begin{eqnarray*}
	\lefteqn{\Pr\left \{\exists k \in [K] \mbox{ such that  } |\hat{\mu}_{n,k}-\widehat{\mu}_{n,k}|\geq \epsilon/4N\right \}} \\  &\leq\sum_{n \in [K]}\Pr\{ |\hat{\mu}_{n,k}-\widehat{\mu}_{n,k}|\geq \epsilon/4N\}\\
	& \leq \sum_{n \in [K]} 2 \exp\left \{- 2T_b(\epsilon/4N)^2 \right \}\\
	&= \sum_{n \in [K]} 2\exp\{-\log(6K^2/\delta)\}= \delta/3K,
\end{eqnarray*}
where the first inequality follows from the union bound, the second from Hoeffding's inequlaity, and the last from substituting value of $T_b$ given in (\ref{eqn:BSLen}). The claim follows by applying union bound over all columns of $\hat{M}$.\hfill\IEEEQED

\section*{Proof of Theorem (\ref{thm:Regret-FS})}
\textbf{Proof i)}\\
We use equation (\ref{eqn:Regret}) to obtain the cumulative regrets in the individual phases. We reduce the notation $R(T,ESER)$ to $R(T)$ for avoiding notation complexity in this proof.

Since we condition of the fact that the RH phase gives an orthogonal assignment, we do not include them in the regret.

In the exploration phase, for every time slot in $KT_s$, the regret will be at the most $\Delta_{max}$. So, $R^{SH}(T) \leq \sum_{l=1}^{l=l_0}\Delta_{max}T_sK = \Delta_{max}T_sKl_0 \leq \Delta_{max}KT_slog(T)$.

The communication phase consists of transmission and reception of estimated rates using packets between players. One can see that in every time slot, we can incur a regret of at most the optimal network reward $\sum_{n \in [N]} \mu_{n, \pi^*(n)} \leq N$. Considering packetized signalling policy $T_b$ = $\lceil log(4N/\epsilon) \rceil$ bits we can bound the regret similarly as shown above to be $R^{BS}(T) \leq \sum_{l=1}^{l=l_0}T_bKN^2 = T_bKN^2l_0 \leq N^2KT_blog(T)$.

%If $\Delta_{min}$ is known, then \sum^{log(T)}_{l=0}2^l\Delta_{max} 
We now consider the regret bound for the exploitation phase. 
\\
Since $\Delta_{min}$ is known, the $\epsilon(l)$ is chosen to be such that $\epsilon(l)<\Delta_{min} \forall l$. Thus the ($\epsilon(l)$,$\delta(l)$)-optimal allocation will give zero regret (corresponding to optimal allocation) with probability $1 - \delta(l)$ and will give a regret of at the most $\Delta_{max}$ with probability $\delta(l)$. 
Therefore, over the $l^{th}$ epoch, this allocation gives a regret of $0$ with probability $1-\delta(l)$ and at the most $\Delta_{max}2^{l}$ with probability $\delta(l)$. Therefore the expected regret over the $l^{th}$ epoch is
\begin{equation}
    R^E(l) \leq 2^{l}\Delta_{max}\delta(l)
\end{equation}
Thus over a period of time $T$, if $l_0$ epochs would have occurred, the cumulative regret would be
\begin{equation}
\begin{array}{lcl}
 R^{E}(T) & = &   \sum^{l_0}_{l=1}R^E(l)\\
          & \leq  & \sum^{l_0}_{l=1}2^{l}(\Delta_{max}\delta(l))\\
          & = & \Delta_{max} \sum^{l_0}_{l=1}2^{l}\delta(l)\\
          & = & \Delta_{max}\sum^{l_0}_{l=1}2^{l}Pr\{ |\hat{M} - M | > \epsilon/2N \}\\
\end{array}
\end{equation}
Using Theorem \ref{thm:DOA-WS} and proof of Lemma \ref{lma:SHPhase},

$Pr\{ |\hat{M} - M | > \epsilon/2N \} = 3/2*Pr\{ \forall n \in [N], \forall k \in [K] \hspace{10pt} |\hat{\mu_{nk}} - \mu_{nk} | > \epsilon/4N \} $
\begin{equation}
\begin{array}{lcl}
          
          & \leq & \Delta_{max}\sum^{l_0}_{l=1}2^{l}*3NKe^{-\epsilon^2lT_s/8N^2}\\
          & \leq & 3NK\Delta_{max}\sum^{l_0}_{l=1}(2e^{-\epsilon^2T_s/8N^2})^{l}\\
          & \leq & 3NK\Delta_{max}\sum^{\infty}_{l=1}(2e^{-\epsilon^2T_s/8N^2})^{l}\\
          & = & C_1NK\Delta_{max}
\end{array}
\end{equation}

Where $C_1 = 6/(e-2)$ and $T_s = 8N^2/\epsilon^2$ for an $\epsilon < \Delta_{min}$

\

\textbf{Proof for ii)} \\
If $\Delta_{min}$ is not known but fixed, we want $\epsilon(l)$ to go below $\Delta_{min}$. This can happen when $\epsilon(l)$ is set to be a decreasing sequence $\epsilon(l) \to 0$ as $l \to \infty$. On doing so we can claim that  $\exists$ $l'$ such that after $l \geq l'$ epochs, $\epsilon(l) \leq \Delta_{min}$ thus always giving an optimal allocation henceforth with probability $\delta(l)$.

Let $t_l$ is the start time of the exploration phase.
We use an increasing sequence of exploration duration i.e. $T_s(l) = log^{(\beta)}(t_l)$ and $\epsilon(l) = log^{-(\beta/2)}(t_l)$ for $\beta \in (0,1)$.
\\

The proof follows a similar structure as that for i).
We consider the exploration phase regret $R^{SH}(T) \leq \sum_{l=1}^{l=l_0}\Delta_{max}T_s(l)K \leq \Delta_{max}Kl_0T_s(l_0) \leq 8N^2K\Delta_{max}log^{(1+\beta)}(T)$

%This is true since if $T_s(l)$ = $log^{\beta}(t_l)$ for $\beta \in (0,1)$, it follows clearly that $log^{(\beta)}t_l \geq l^{(\beta)}$. Then, $\sum_{l=1}^{l=l_0}T_s(l) \geq \sum_{l=1}^{l=l_0}l^{(\beta)} \geq \int_{x=1}^{x=l_0+1}(x-1)^{\beta} dx \geq 0.5l_0^{(1+\beta)}$ 

Next we consider the signalling phase regret bound. 
By definition, 
\begin{equation}
\begin{array}{lcl}
T_b(l) 
& = & \lceil log_2(4N/(\epsilon(l)) \rceil \\
&= & \lceil log_2(4N*log^{\beta/2)}(t_l)) \rceil\\
& = & log_2(4N) +log_2(log^{(\beta/2)}(t_l)) \hfill{\because}\\
& \leq & log_2(4N)  + log^{(\beta/2)}(t_l)
\end{array}
\end{equation}
So, the upper bound on the cumulative regret in the signalling phases is given as follows:

\begin{equation}
\begin{array}{lcl}
R^{BS}(T) 
& \leq &  \sum_{l=1}^{l=l_0}T_b(l) KN^2 \\
& = &  N^2K \sum_{l=1}^{l=l_0}T_b(l) \\
& \leq & C_4 \sum_{l=1}^{l=l_0}log^{(\beta/2)}(t_l) + C_5l_0\\
&  \leq & C_4\sum_{l=1}^{l=l_0}log^{(\beta/2)}(t_{l_0}) + C_5l_0\\
&  \leq & C_4l_0log^{(\beta/2)}(t_{l_0}) + C_5l_0\\
&  \leq & C_4log(T)log^{(\beta/2)}(t_{l_0}) + C_5log(T)\\
&  \leq & C_4log(T)log^{(\beta/2)}(T) + C_5log(T)\\
&  \leq & C_4log^{(1+\beta/2)}(T) + C_5log(T)\\
\end{array}
\end{equation}

where $C_4 = N^2K$ and $C_5 =  N^2Klog_2(4N)$

We now look at the regret in the exploitation phase. The proof is similar to i), with a change that the value of $\Delta_{min}$ is not known. Hence, the ($\epsilon(l)$,$\delta(l)$)-optimal allocation will give at the most $\epsilon(l)$ regret with probability $1 - \delta(l)$ and will give a regret of at the most $\Delta_{max}$ with probability $\delta(l)$. Thus over the $l^{th}$ epoch, the expected regret would be $R^E(l) = 2^{l}(\epsilon(l)(1-\delta(l) + \Delta_{max}\delta(l))$

Therefore, the cumulative expected regret in the exploitation phase is as follows: 
\begin{equation}
\begin{array}{lcl}
 R^{E}(T) & = &   \sum^{l_0}_{l=1}R^E(l)\\
          & \leq  & \sum^{l_0}_{l=1}2^{l}(\epsilon(l)(1-\delta(l) + \Delta_{max}\delta(l))\\
          & = & \sum^{l_0}_{l=1}2^{l}(\epsilon(l)+\delta(l)(\Delta_{max}-\epsilon(l)))\\
\end{array}
\end{equation}
Since $\epsilon(l)$ is monotonically decreasing, there exists a finite $l'$ such that $\forall l >l', \epsilon(l) < \Delta_{min}$. Thus the cumulative regret now becomes
\begin{equation}
\begin{array}{lcl}
R^{E}(T)        
          & = & \sum^{l'}_{l=1}2^{l}(\epsilon(l)+\delta(l)(\Delta_{max}-\epsilon(l)))\\  
          &  & \hspace{30pt} + \sum^{l_0}_{l=l'}2^{l}\delta(l)\Delta_{max} \\
          & = & \sum^{l'}_{l=1}2^{l}(\epsilon(l)+\delta(l)(\Delta_{max}-\epsilon(l)))\\  
          &  & \hspace{30pt} + \Delta_{max}\sum^{l_0}_{l=l'}2^lPr\{ |\hat{M}(l)-M|>\epsilon(l)/2N  \} \\
\end{array}
\end{equation}

Using Theorem \ref{thm:DOA-WS} and proof of Lemma \ref{lma:SHPhase},

$Pr\{ |\hat{M} - M | > \epsilon(l)/2N \} = 3/2*Pr\{ \forall n \in [N], \forall k \in [K] \hspace{10pt} |\hat{\mu_{nk}} - \mu_{nk} | > \epsilon(l)/4N \} $

Upon evaluating the first of the two summations, we get 
\begin{equation}
\begin{array}{lcl}

 R^E_1(T) &=  &\sum^{l'}_{l=1}2^{l}\epsilon(l)+ 2^l\delta(l)(\Delta_{max}-\epsilon(l)) \\

& \leq & \sum^{l'}_{l=1}2^{l}\epsilon(1) + 2^l\delta(1)\Delta_{max} \\

& \leq & \sum^{l'}_{l=1}2^{l}(\epsilon(1) + \delta(1)\Delta_{max}) \\

& \leq & 2^{l'+1}(\epsilon(1) + \delta(1)\Delta_{max}) \\

& \leq & 2^{l'+1}(1 + \Delta_{max})\\
& = & C_2

\end{array}
\end{equation}
The last step comes from the fact that true mean rewards are bounded by $1$ and hence an initial $\epsilon$ should be chosen below that only. Further, $\delta$ being the error probability of ($\epsilon,\delta$) optimal assignment, is chosen less than $1$.

The second of the two summations can be bounded as follows:
\begin{equation}
\begin{array}{lcl}
R^E_2(T)&= & \Delta_{max}\sum^{l_0}_{l=l'}2^lPr\{ |\hat{M}(l)>M|>\epsilon(l)/2N  \}\\
& \leq & \Delta_{max}\sum^{l_0}_{l=l'}2^{l}*3NKe^{-\epsilon(l)^2lT_s(l)/8N^2}\\
& \leq & 3NK\Delta_{max}\sum^{l_0}_{l=l'}(2e^{-\epsilon^2T_s/8N^2})^{l}\\
& \leq & 3NK\Delta_{max}\sum^{l_0}_{l=l'}(2e^{-1})^{l}\\
& \leq & 3NK\Delta_{max}\sum^{\infty}_{l=l'}(2e^{-1})^{l}\\
& = & C_3NK\Delta_{max}
\end{array}
\end{equation}

where $C_3 = 3r^{l'}/(1-r)$ where $r=2e^{-1}$.

Since, $R^E(T) = R^E_1(T) + R^E_2(T)$, exploitation regret turns out to be independent of T. \hfill\IEEEQED

\section*{Proof of Lemma \ref{lma:secondAlloc}}
Let $\hat{M}(l)$ be the estimated matrix after learning and signalling in the $l_{th}$ epoch. Let $\hat{\pi}_1(l) \in A(\hat{M}(l))$ and $\hat{\pi}_2(l) \in \bar{A}(\hat{M}(l))$ be a best and a second-best allocations on $\hat{M}(l)$ respectively. Similarly, let $\pi_1$ and $\pi_2$ be similar quantities in case of the matrix $M$.
Also, we define $\hat{\Delta}_{min}(l) = f(\hat{M}(l),\hat{\pi}_1(l)) - f(\hat{M}(l),\hat{\pi}_2(l))$, which turns out to be what every player estimates $\Delta_{min}$ as.

\textit{Case 1 : If $\pi_1=\hat{\pi}_1$}
\begin{equation*}
f(\hat{M},\hat{\pi}_2) \leq f(M+I\epsilon,\hat{\pi}_2) \leq f(M+I\epsilon,\pi_2)
\end{equation*}   
where the second inequality holds because $\pi_1=\hat{\pi}_1 \neq \hat{\pi}_2$ and thus $\hat{\pi}_2$ cannot give better reward on $M$ than $\pi_2$. 

\textit{Case 2 : If $\pi_1 \neq \hat{\pi}_1$}
\begin{equation*}
f(\hat{M},\hat{\pi}_2) \leq f(\hat{M},\hat{\pi}_1) \leq f(M+I\epsilon,\hat{\pi}_1) \leq f(M+I\epsilon,\pi_2)
\end{equation*}   
where the third inequality holds because $\pi_1 \neq \hat{\pi}_1$ and thus $\hat{\pi}_1$ cannot give better reward on $M$ than $\pi_2$.
We also know that $f(M+I\epsilon,\pi_2) = f(M,\pi_2)+N\epsilon$. Thus we have shown that $f(\hat{M},\hat{\pi}_2) - f(M,\pi_2) \leq N\epsilon$

To prove the other side of the inequality 

\textit{Case 1: If $\pi_1=\hat{\pi}_1$}
\begin{equation*}
f(M-I\epsilon,\pi_2) \leq f(\hat{M},\pi_2) \leq f(\hat{M},\hat{\pi}_2)
\end{equation*}   
where the last inequality holds because $\pi_1=\hat{\pi}_1 \neq \pi_2$ and thus $\pi_2$ cannot give better reward on $\hat{M}$ than $\hat{\pi}_2$. 
\textit{Case 2 : If $\pi_1 \neq \hat{\pi}_1$}
\begin{equation*}
f(M-I\epsilon,\pi_2) \leq f(M-I\epsilon,\pi_1) \leq f(\hat{M},\pi_1) \leq f(\hat{M},\hat{\pi_2})
\end{equation*}
where the last inequality holds because $\pi_1 \neq \hat{\pi}_1$ and thus $\pi_1$ cannot give better reward on $\hat{M}$ than $\hat{\pi}_2$. 
We also know that $f(M-I\epsilon,\pi_2) =  f(M,\pi_2)-N\epsilon$. Thus we have shown that $-N\epsilon \leq f(\hat{M},\hat{\pi}_2) - f(M,\pi_2)$.

From equation (\ref{eqn:perturb2}) and from lemma (\ref{lma:secondAlloc}), we know
\begin{gather}
-N\epsilon \leq f(M,\pi_1) - f(\hat{M},\hat{\pi}_1) \leq N\epsilon \\ 
-N\epsilon \leq f(M,\pi_2) - f(\hat{M},\hat{\pi}_2) \leq N\epsilon 
\end{gather}

Subtracting the above two inequalities and rearranging terms, we obtain
\begin{equation*}
-2N\epsilon \leq \Delta_{min} - \hat{\Delta}_{min} \leq 2N\epsilon   
\end{equation*}
\hfill \IEEEQED

\section*{Proof of Theorem (\ref{thm:mESER})}
 
We continue to prove the regret bound similar to the way it was done for Theorem \ref{thm:Regret-FS}. We provide bounds on the regret in the 3 phases namely exploration ($R^{0}(T)$) , signalling($R^{S}(T)$) and exploitation($R^{E}(T)$). 

In the exploration phase, every epoch has $T_s(l) = 8N^2log^{(\beta)}(t_l)$ time slots till the $l_1^{th}$ epoch after which it is a constant, giving a total regret of 
\begin{equation}
\begin{array}{lcl}
R^O(T) 
& \leq& \sum_{l=1}^{l=l_0} \Delta_{max} T_s(l)K  \\
&= &\sum_{l=1}^{l=l_1} \Delta_{max} T_s(l)K + \sum_{l=l_1+1}^{l=l_0} \Delta_{max} T_s(l_1)K\\
& \leq & \Delta_{max}Klog(t_{l_1})T_s(l_1) +\Delta_{max} T_0Kl_0 \\
& \leq & \Delta_{max}Klog(t_{l_1})T_s(l_1) +\Delta_{max} T_0Klog(T) \\
& \leq & \Delta_{max}KC_1 +\Delta_{max} T_0Klog(T) \\
\end{array}
\end{equation}

Similarly for the signalling phase, we consider packetized transmission. If $T_b(l) = \lceil log_2(4N/(\epsilon(l)) \rceil$, from Equation (\ref{e}) we have $T_b(l) \leq log_{2}(4N) + log^{\beta/2}(t_l)$. Thus we have the regret in the communication phase as  
\begin{equation*}
\begin{array}{lcl}
R^{S}(T) 
& \leq &  \sum_{l=1}^{l=l_0}T_b(l) KN^2 \\
& = &  N^2K \sum_{l=1}^{l=l_0}T_b(l) \\
& \leq & N^2K \sum_{l=1}^{l=l_1}T_b(l) + N^2K \sum_{l=l_1}^{l=l_0}T_b(l_1) \\
\end{array}
\end{equation*}
Once the $l_i$ epoch is completed, $T_b(l) =T_1=\lceil log_2(4N/(\epsilon_0) \rceil$  $\forall l > l_1$

\begin{equation*}
\begin{array}{lcl}
R^{S}(T)
&  \leq & N^2K( log_2(4N)l_1 + log^{(1+\beta)}(t_{l_1})) + N^2KT_1l_0  \\
&  \leq & N^2K( log_2(4N)l_1 + log^{(1+\beta)}(t_{l_1})) + N^2KT_1log(T)  \\
&  = & N^2KC_2 + N^2KT_1log(T)  \\
\end{array}
\end{equation*}

We now look the regret in the exploitation phase. From Equation () we have:

\begin{equation}
    \begin{array}{lcl}
    R^{E}(T) 
    & = &   \sum^{l_0}_{l=1}R^E(l)\\
    & = & \sum^{l_0}_{l=1}2^{l}(\epsilon(l)+\delta(l)(\Delta_{max}-\epsilon(l)))\\
    & = & \sum^{l_1}_{l=1}2^{l}(\epsilon(l)+\delta(l)(\Delta_{max}-\epsilon(l)))\\
    &  & + \Delta_{max}\sum^{l_0}_{l=l_1}2^{l}\delta(l)\\
    & = & R^{E}_1(T) + R^{E}_2(T)
    \end{array}
\end{equation}

We split $R^E(T)$ in two terms

\begin{equation}
    \begin{array}{lcl}
    R^{E}_1(T) 
    & = & \sum^{l_1}_{l=1}2^{l}(\epsilon(l)+\delta(l)(\Delta_{max}-\epsilon(l)))\\
    & \leq & 2^{l_1+1}(1+\Delta_{max}) \\
    & = & C_3
    \end{array}
\end{equation}
Since after $l_1$ epochs, we set $\epsilon(l) = \epsilon_0$
\begin{equation}
\begin{array}{lcl}
R^E_2(T)&= & \Delta_{max}\sum^{l_0}_{l=l_1}2^l\delta(l) \\
&= & \Delta_{max}\sum^{l_0}_{l=l_1}2^lPr\{ |\hat{M}(l)>M|>\epsilon(l)/2N  \}\\
& \leq & \Delta_{max}\sum^{l_0}_{l=l'}2^{l}*3NKe^{-\epsilon(l)^2lT_s/8N^2}\\
& \leq & 3NK\Delta_{max}\sum^{l_0}_{l=l_1}(2e^{-\epsilon^2T_s/8N^2})^{l}\\
& \leq & 3NK\Delta_{max}\sum^{l_0}_{l=l_1}(2e^{-1})^{l}\\
& \leq & 3NK\Delta_{max}\sum^{\infty}_{l=l_1}(2e^{-1})^{l}\\
& = & C_4NK\Delta_{max}
\end{array}
\end{equation}

where $C_4 = 3r^{l_1}/(1-r)$ where $r=2e^{-1}$.
